# Supplementary material for: Traffic Context Aware Data Augmentation for Rare Object Detection in Autonomous Driving
Source: arXiv:2205.00376 source file (2022-07-02)
Supplement: Supplementary file 1 [file appendix.tex]

% --- architecture details
\subsection{NM10K}
\label{sec:nu10k}
In this section, we present additional details regarding NM10k dataset.
